# Supplementary material for: The hadronic vacuum polarization and automatic O(a) improvement for twisted mass fermions
Source: arXiv:1412.0546 ancillary file (2015-03-23)
Supplement: Supplementary file 1 [file non_derivative_symtranstab.pdf]

| dim. | type | subtype | operator                      | $\mathcal{P}_{1/2}$ | $\mathcal{P}[-\mu]$ | $\mathcal{T}_{1/2}$ | $\mathcal{T}[-\mu]$ | $\mathcal{C}$ | $\mathcal{PD}[-m][-r]$ | $\mathcal{R}_5^{1/2}\mathcal{D}[-\mu]$ |
|------|------|---------|-------------------------------|---------------------|---------------------|---------------------|---------------------|---------------|------------------------|----------------------------------------|
| 0    |      |         | $\mathbb{1}$                  | +1                  | +1                  | +1                  | +1                  | +1            | +1                     | +1                                     |
|      |      |         | $r\mathbb{1}$                 | +1                  | +1                  | +1                  | +1                  | +1            | -1                     | +1                                     |
| 1    | 1    | 1       | $m_q$                         | +1                  | +1                  | +1                  | +1                  | +1            | -1                     | +1                                     |
|      |      |         | $rm_q$                        | +1                  | +1                  | +1                  | +1                  | +1            | +1                     | +1                                     |
|      | 2    | 2       | $\mu_q$                       | +1                  | -1                  | +1                  | -1                  | +1            | +1                     | -1                                     |
|      |      |         | $r\mu_q$                      | +1                  | -1                  | +1                  | -1                  | +1            | -1                     | -1                                     |
| 2    | 1    | 1       | $m_q^2$                       | +1                  | +1                  | +1                  | +1                  | +1            | +1                     | +1                                     |
|      |      |         | $rm_q^2$                      | +1                  | +1                  | +1                  | +1                  | +1            | -1                     | +1                                     |
|      | 2    | 2       | $m_q\mu_q$                    | +1                  | -1                  | +1                  | -1                  | +1            | -1                     | -1                                     |
|      |      |         | $rm_q\mu_q$                   | +1                  | -1                  | +1                  | -1                  | +1            | +1                     | -1                                     |
|      | 3    | 3       | $\mu_q^2$                     | +1                  | +1                  | +1                  | +1                  | +1            | +1                     | +1                                     |
|      |      |         | $r\mu_q^2$                    | +1                  | +1                  | +1                  | +1                  | +1            | -1                     | +1                                     |
| 3    | 1    | 1       | $m_q^3$                       | +1                  | +1                  | +1                  | +1                  | +1            | -1                     | +1                                     |
|      |      |         | $rm_q^3$                      | +1                  | +1                  | +1                  | +1                  | +1            | +1                     | +1                                     |
|      |      |         | $m_q^2\mu_q$                  | +1                  | -1                  | +1                  | -1                  | +1            | +1                     | -1                                     |
|      |      |         | $rm_q^2\mu_q$                 | +1                  | -1                  | +1                  | -1                  | +1            | -1                     | -1                                     |
|      | 3    | 3       | $m_q\mu_q^2$                  | +1                  | +1                  | +1                  | +1                  | +1            | -1                     | +1                                     |
|      |      |         | $rm_q\mu_q^2$                 | +1                  | +1                  | +1                  | +1                  | +1            | +1                     | +1                                     |
|      | 4    | 4       | $\mu_q^3$                     | +1                  | -1                  | +1                  | -1                  | +1            | +1                     | -1                                     |
|      |      |         | $r\mu_q^3$                    | +1                  | -1                  | +1                  | -1                  | +1            | -1                     | -1                                     |
|      | 2    | 1       | $\bar{\chi}(y)\chi(y)$        | +1                  | +1                  | +1                  | +1                  | +1            | -1                     | +1                                     |
|      |      |         | $r\bar{\chi}(y)\chi(y)$       | +1                  | +1                  | +1                  | +1                  | +1            | +1                     | +1                                     |
|      | 2    | 2       | $\bar{\chi}(y)\tau^3\chi(y)$  | -1                  | +1                  | -1                  | +1                  | +1            | -1                     | -1                                     |
|      |      |         | $r\bar{\chi}(y)\tau^3\chi(y)$ | -1                  | +1                  | -1                  | +1                  | +1            | +1                     | -1                                     |

|   |   |   |   |                                                             |                                           |               |               |               |    |               |    |
|---|---|---|---|-------------------------------------------------------------|-------------------------------------------|---------------|---------------|---------------|----|---------------|----|
|   |   |   |   |                                                             | $\bar{\chi}(y) \gamma_5 \chi(y)$          | -1            | -1            | -1            | +1 | +1            | +1 |
|   |   |   |   |                                                             | $r \bar{\chi}(y) \gamma_5 \chi(y)$        | -1            | -1            | -1            | -1 | -1            | +1 |
|   |   |   |   |                                                             | $\bar{\chi}(y) \gamma_5 \tau^3 \chi(y)$   | +1            | -1            | -1            | +1 | +1            | -1 |
|   |   |   |   |                                                             | $r \bar{\chi}(y) \gamma_5 \tau^3 \chi(y)$ | +1            | -1            | +1            | +1 | -1            | -1 |
| 4 | 1 | 3 | 1 | $m_q \bar{\chi}(y) \chi(y)$                                 | +1                                        | +1            | +1            | +1            | +1 | +1            | +1 |
|   |   |   |   | $r m_q \bar{\chi}(y) \chi(y)$                               | +1                                        | +1            | +1            | +1            | +1 | +1            | +1 |
|   |   |   |   | $m_q \bar{\chi}(y) \tau^3 \chi(y)$                          | -1                                        | +1            | -1            | +1            | +1 | -1            | -1 |
|   |   |   |   | $r m_q \bar{\chi}(y) \tau^3 \chi(y)$                        | -1                                        | +1            | -1            | +1            | +1 | -1            | -1 |
|   |   |   |   | $m_q \bar{\chi}(y) \gamma_5 \chi(y)$                        | -1                                        | -1            | -1            | -1            | +1 | +1            | +1 |
|   |   |   |   | $r m_q \bar{\chi}(y) \gamma_5 \chi(y)$                      | -1                                        | -1            | -1            | -1            | +1 | +1            | +1 |
|   |   |   |   | $m_q \bar{\chi}(y) \gamma_5 \tau^3 \chi(y)$                 | +1                                        | -1            | +1            | -1            | +1 | -1            | -1 |
|   |   |   |   | $r m_q \bar{\chi}(y) \gamma_5 \tau^3 \chi(y)$               | +1                                        | -1            | +1            | -1            | +1 | -1            | -1 |
|   | 2 | 1 | 1 | $\mu_q \bar{\chi}(y) \chi(y)$                               | +1                                        | -1            | +1            | -1            | +1 | -1            | -1 |
|   |   |   |   | $r \mu_q \bar{\chi}(y) \chi(y)$                             | +1                                        | -1            | +1            | -1            | +1 | -1            | -1 |
|   |   |   |   | $\mu_q \bar{\chi}(y) \tau^3 \chi(y)$                        | -1                                        | -1            | -1            | -1            | +1 | +1            | +1 |
|   |   |   |   | $r \mu_q \bar{\chi}(y) \tau^3 \chi(y)$                      | -1                                        | -1            | -1            | -1            | +1 | +1            | +1 |
|   |   |   |   | $\mu_q \bar{\chi}(y) \gamma_5 \chi(y)$                      | -1                                        | +1            | -1            | +1            | +1 | -1            | -1 |
|   |   |   |   | $r \mu_q \bar{\chi}(y) \gamma_5 \chi(y)$                    | -1                                        | +1            | -1            | +1            | +1 | -1            | -1 |
|   |   |   |   | $\mu_q \bar{\chi}(y) \gamma_5 \tau^3 \chi(y)$               | +1                                        | +1            | +1            | +1            | +1 | +1            | +1 |
|   |   |   |   | $r \mu_q \bar{\chi}(y) \gamma_5 \tau^3 \chi(y)$             | +1                                        | +1            | +1            | +1            | +1 | +1            | +1 |
|   | 3 | 1 | 1 | $\text{tr} [C_{\mu\lambda}(y) C_{\lambda\nu}(y)]$           | $I_{\mu\nu}$                              | $I_{\mu\nu}$  | $I_{\mu\nu}$  | $I_{\mu\nu}$  | +1 | $I_{\mu\nu}$  | +1 |
|   |   |   |   | $r \text{tr} [C_{\mu\lambda}(y) C_{\lambda\nu}(y)]$         | $I_{\mu\nu}$                              | $I_{\mu\nu}$  | $I_{\mu\nu}$  | $I_{\mu\nu}$  | +1 | $-I_{\mu\nu}$ | +1 |
|   |   |   |   | $\text{tr} [C_{\mu\lambda}(y) \tilde{C}_{\lambda\nu}(y)]$   | $-I_{\mu\nu}$                             | $-I_{\mu\nu}$ | $-I_{\mu\nu}$ | $-I_{\mu\nu}$ | +1 | $-I_{\mu\nu}$ | +1 |
|   |   |   |   | $r \text{tr} [C_{\mu\lambda}(y) \tilde{C}_{\lambda\nu}(y)]$ | $-I_{\mu\nu}$                             | $-I_{\mu\nu}$ | $-I_{\mu\nu}$ | $-I_{\mu\nu}$ | +1 | $+I_{\mu\nu}$ | +1 |
|   | 4 | 1 |   | $m_q^4$                                                     | +1                                        | +1            | +1            | +1            | +1 | +1            | +1 |





|   |   |   |   |   |                                                                  |  |               |               |               |               |    |
|---|---|---|---|---|------------------------------------------------------------------|--|---------------|---------------|---------------|---------------|----|
|   | 6 |   |   |   | $r\mu_q^5$                                                       |  | +1            | -1            | +1            | -1            | -1 |
|   |   | 1 |   |   | $m_q \text{tr} [C_{\mu\lambda}(y) C_{\lambda\nu}(y)]$            |  | $I_{\mu\nu}$  | $I_{\mu\nu}$  | $I_{\mu\nu}$  | $-I_{\mu\nu}$ | +1 |
|   |   | 2 |   |   | $rm_q \text{tr} [C_{\mu\lambda}(y) C_{\lambda\nu}(y)]$           |  | $I_{\mu\nu}$  | $I_{\mu\nu}$  | $I_{\mu\nu}$  | $I_{\mu\nu}$  | +1 |
|   |   |   | 2 |   | $m_q \text{tr} [C_{\mu\lambda}(y) \tilde{C}_{\lambda\nu}(y)]$    |  | $-I_{\mu\nu}$ | $-I_{\mu\nu}$ | $-I_{\mu\nu}$ | $I_{\mu\nu}$  | +1 |
|   |   |   | 3 |   | $rm_q \text{tr} [C_{\mu\lambda}(y) \tilde{C}_{\lambda\nu}(y)]$   |  | $-I_{\mu\nu}$ | $-I_{\mu\nu}$ | $-I_{\mu\nu}$ | $-I_{\mu\nu}$ | +1 |
|   |   |   |   | 3 | $\mu_q \text{tr} [C_{\mu\lambda}(y) C_{\lambda\nu}(y)]$          |  | $I_{\mu\nu}$  | $-I_{\mu\nu}$ | $I_{\mu\nu}$  | $I_{\mu\nu}$  | -1 |
|   |   |   |   | 4 | $r\mu_q \text{tr} [C_{\mu\lambda}(y) C_{\lambda\nu}(y)]$         |  | $I_{\mu\nu}$  | $-I_{\mu\nu}$ | $-I_{\mu\nu}$ | $-I_{\mu\nu}$ | -1 |
|   |   |   |   |   | $\mu_q \text{tr} [C_{\mu\lambda}(y) \tilde{C}_{\lambda\nu}(y)]$  |  | $-I_{\mu\nu}$ | $I_{\mu\nu}$  | $-I_{\mu\nu}$ | $-I_{\mu\nu}$ | -1 |
|   |   |   |   |   | $r\mu_q \text{tr} [C_{\mu\lambda}(y) \tilde{C}_{\lambda\nu}(y)]$ |  | $-I_{\mu\nu}$ | $-I_{\mu\nu}$ | $I_{\mu\nu}$  | $I_{\mu\nu}$  | -1 |
| 6 | 1 | 1 |   |   | $m_q^3 \bar{\chi}(y) \chi(y)$                                    |  | +1            | +1            | +1            | +1            | +1 |
|   |   | 2 |   |   | $rm_q^3 \bar{\chi}(y) \chi(y)$                                   |  | +1            | +1            | +1            | +1            | +1 |
|   |   |   | 2 |   | $m_q^3 \bar{\chi}(y) \tau^3 \chi(y)$                             |  | -1            | +1            | +1            | +1            | -1 |
|   |   |   | 3 |   | $rm_q^3 \bar{\chi}(y) \tau^3 \chi(y)$                            |  | -1            | +1            | +1            | +1            | -1 |
|   |   |   |   | 3 | $m_q^3 \bar{\chi}(y) \gamma_5 \chi(y)$                           |  | -1            | -1            | -1            | -1            | +1 |
|   |   |   |   | 4 | $rm_q^3 \bar{\chi}(y) \gamma_5 \chi(y)$                          |  | -1            | -1            | -1            | +1            | +1 |
|   |   |   |   |   | $m_q^3 \bar{\chi}(y) \gamma_5 \tau^3 \chi(y)$                    |  | +1            | -1            | +1            | -1            | -1 |
|   |   |   |   |   | $rm_q^3 \bar{\chi}(y) \gamma_5 \tau^3 \chi(y)$                   |  | +1            | -1            | +1            | +1            | -1 |
|   | 2 | 1 |   |   | $m_q^2 \mu_q \bar{\chi}(y) \chi(y)$                              |  | +1            | -1            | +1            | -1            | -1 |
|   |   |   | 2 |   | $rm_q^2 \mu_q \bar{\chi}(y) \chi(y)$                             |  | +1            | -1            | +1            | +1            | -1 |
|   |   |   |   | 2 | $m_q^2 \mu_q \bar{\chi}(y) \tau^3 \chi(y)$                       |  | -1            | -1            | -1            | -1            | +1 |
|   |   |   |   | 3 | $rm_q^2 \mu_q \bar{\chi}(y) \tau^3 \chi(y)$                      |  | -1            | -1            | -1            | +1            | +1 |
|   |   |   |   |   | $m_q^2 \mu_q \bar{\chi}(y) \gamma_5 \chi(y)$                     |  | -1            | +1            | +1            | +1            | -1 |
|   |   |   |   | 4 | $rm_q^2 \mu_q \bar{\chi}(y) \gamma_5 \chi(y)$                    |  | -1            | +1            | +1            | -1            | -1 |
|   |   |   |   |   | $m_q^2 \mu_q \bar{\chi}(y) \gamma_5 \tau^3 \chi(y)$              |  | +1            | +1            | +1            | +1            | +1 |



|    |   |  | $rm_q \mu_q \text{tr} [C_{\mu\lambda}(y) \tilde{C}_{\lambda\nu}(y)]$            | $-I_{\mu\nu}$ | $I_{\mu\nu}$  | $-I_{\mu\nu}$ | $I_{\mu\nu}$  | $-I_{\mu\nu}$ | $-I_{\mu\nu}$ | $-I_{\mu\nu}$ |
|----|---|--|---------------------------------------------------------------------------------|---------------|---------------|---------------|---------------|---------------|---------------|---------------|
| 5  |   |  | $\mu_q^2 \text{tr} [C_{\mu\lambda}(y) C_{\lambda\nu}(y)]$                       | $I_{\mu\nu}$  | $I_{\mu\nu}$  | $I_{\mu\nu}$  | $I_{\mu\nu}$  | $I_{\mu\nu}$  | $I_{\mu\nu}$  | $-1$          |
| 6  |   |  | $r \mu_q^2 \text{tr} [C_{\mu\lambda}(y) C_{\lambda\nu}(y)]$                     | $I_{\mu\nu}$  | $I_{\mu\nu}$  | $I_{\mu\nu}$  | $I_{\mu\nu}$  | $I_{\mu\nu}$  | $I_{\mu\nu}$  | $+1$          |
|    |   |  | $\mu_q^2 \text{tr} [C_{\mu\lambda}(y) \tilde{C}_{\lambda\nu}(y)]$               | $-I_{\mu\nu}$ | $-I_{\mu\nu}$ | $-I_{\mu\nu}$ | $-I_{\mu\nu}$ | $-I_{\mu\nu}$ | $-I_{\mu\nu}$ | $+1$          |
|    |   |  | $r \mu_q^2 \text{tr} [C_{\mu\lambda}(y) \tilde{C}_{\lambda\nu}(y)]$             | $-I_{\mu\nu}$ | $-I_{\mu\nu}$ | $-I_{\mu\nu}$ | $-I_{\mu\nu}$ | $-I_{\mu\nu}$ | $-I_{\mu\nu}$ | $+1$          |
| 1  | 6 |  | $\bar{\chi}(y) \chi(y) \bar{\chi}(y) \chi(y)$                                   | $+1$          | $+1$          | $+1$          | $+1$          | $+1$          | $+1$          | $+1$          |
| 2  |   |  | $r \bar{\chi}(y) \chi(y) \bar{\chi}(y) \chi(y)$                                 | $+1$          | $+1$          | $+1$          | $+1$          | $+1$          | $+1$          | $+1$          |
|    |   |  | $\bar{\chi}(y) \chi(y) \bar{\chi}(y) \tau^3 \chi(y)$                            | $-1$          | $+1$          | $-1$          | $+1$          | $+1$          | $+1$          | $-1$          |
| 3  |   |  | $r \bar{\chi}(y) \chi(y) \bar{\chi}(y) \tau^3 \chi(y)$                          | $-1$          | $+1$          | $-1$          | $+1$          | $+1$          | $+1$          | $-1$          |
|    |   |  | $\bar{\chi}(y) \tau^3 \chi(y) \bar{\chi}(y) \tau^3 \chi(y)$                     | $+1$          | $+1$          | $+1$          | $+1$          | $+1$          | $+1$          | $+1$          |
| 4  |   |  | $r \bar{\chi}(y) \tau^3 \chi(y) \bar{\chi}(y) \tau^3 \chi(y)$                   | $+1$          | $+1$          | $+1$          | $+1$          | $+1$          | $+1$          | $+1$          |
|    |   |  | $\bar{\chi}(y) \chi(y) \bar{\chi}(y) \gamma_5 \chi(y)$                          | $-1$          | $-1$          | $-1$          | $-1$          | $-1$          | $-1$          | $+1$          |
| 5  |   |  | $r \bar{\chi}(y) \chi(y) \bar{\chi}(y) \gamma_5 \chi(y)$                        | $-1$          | $-1$          | $-1$          | $-1$          | $-1$          | $-1$          | $+1$          |
|    |   |  | $\bar{\chi}(y) \chi(y) \bar{\chi}(y) \gamma_5 \tau^3 \chi(y)$                   | $+1$          | $-1$          | $+1$          | $-1$          | $+1$          | $-1$          | $-1$          |
| 6  |   |  | $r \bar{\chi}(y) \chi(y) \bar{\chi}(y) \gamma_5 \tau^3 \chi(y)$                 | $+1$          | $-1$          | $+1$          | $-1$          | $+1$          | $-1$          | $-1$          |
|    |   |  | $\bar{\chi}(y) \tau^3 \chi(y) \bar{\chi}(y) \gamma_5 \chi(y)$                   | $+1$          | $-1$          | $+1$          | $-1$          | $+1$          | $-1$          | $-1$          |
| 7  |   |  | $r \bar{\chi}(y) \tau^3 \chi(y) \bar{\chi}(y) \gamma_5 \chi(y)$                 | $+1$          | $-1$          | $+1$          | $-1$          | $+1$          | $-1$          | $-1$          |
|    |   |  | $\bar{\chi}(y) \tau^3 \chi(y) \bar{\chi}(y) \gamma_5 \tau^3 \chi(y)$            | $-1$          | $-1$          | $-1$          | $-1$          | $-1$          | $-1$          | $+1$          |
| 8  |   |  | $r \bar{\chi}(y) \tau^3 \chi(y) \bar{\chi}(y) \gamma_5 \tau^3 \chi(y)$          | $-1$          | $-1$          | $-1$          | $-1$          | $-1$          | $-1$          | $+1$          |
|    |   |  | $\bar{\chi}(y) \gamma_5 \chi(y) \bar{\chi}(y) \gamma_5 \chi(y)$                 | $+1$          | $+1$          | $+1$          | $+1$          | $+1$          | $+1$          | $+1$          |
| 9  |   |  | $r \bar{\chi}(y) \gamma_5 \chi(y) \bar{\chi}(y) \gamma_5 \chi(y)$               | $+1$          | $+1$          | $+1$          | $+1$          | $+1$          | $+1$          | $+1$          |
|    |   |  | $\bar{\chi}(y) \gamma_5 \chi(y) \bar{\chi}(y) \gamma_5 \tau^3 \chi(y)$          | $-1$          | $+1$          | $-1$          | $+1$          | $+1$          | $+1$          | $-1$          |
| 10 |   |  | $r \bar{\chi}(y) \gamma_5 \chi(y) \bar{\chi}(y) \gamma_5 \tau^3 \chi(y)$        | $-1$          | $+1$          | $-1$          | $+1$          | $+1$          | $+1$          | $-1$          |
|    |   |  | $\bar{\chi}(y) \gamma_5 \tau^3 \chi(y) \bar{\chi}(y) \gamma_5 \tau^3 \chi(y)$   | $+1$          | $+1$          | $+1$          | $+1$          | $+1$          | $+1$          | $+1$          |
|    |   |  | $r \bar{\chi}(y) \gamma_5 \tau^3 \chi(y) \bar{\chi}(y) \gamma_5 \tau^3 \chi(y)$ | $+1$          | $+1$          | $+1$          | $+1$          | $+1$          | $+1$          | $+1$          |





|  |    |   |   |                                                                                                                                                                                                                                                                                                                                                                                                                                                                                                                                                                                                                                                                                                                                                        |                                                                                                                                                              |                                                                                                                                                                      |                                                                                                                                                                      |                                                                              |                                                                                                                                                                     |                                                                              |
|--|----|---|---|--------------------------------------------------------------------------------------------------------------------------------------------------------------------------------------------------------------------------------------------------------------------------------------------------------------------------------------------------------------------------------------------------------------------------------------------------------------------------------------------------------------------------------------------------------------------------------------------------------------------------------------------------------------------------------------------------------------------------------------------------------|--------------------------------------------------------------------------------------------------------------------------------------------------------------|----------------------------------------------------------------------------------------------------------------------------------------------------------------------|----------------------------------------------------------------------------------------------------------------------------------------------------------------------|------------------------------------------------------------------------------|---------------------------------------------------------------------------------------------------------------------------------------------------------------------|------------------------------------------------------------------------------|
|  |    |   | 4 | $rm_q \bar{\chi}(y) \sigma_{\mu\lambda} \gamma_5 C_{\lambda\nu}(y) \chi(y)$<br>$m_q \bar{\chi}(y) \sigma_{\mu\lambda} \gamma_5 \tau^3 C_{\lambda\nu}(y) \chi(y)$<br>$rm_q \bar{\chi}(y) \sigma_{\mu\lambda} \gamma_5 \tau^3 C_{\lambda\nu}(y) \chi(y)$                                                                                                                                                                                                                                                                                                                                                                                                                                                                                                 | $-I_{\mu\nu}$<br>$I_{\mu\nu}$<br>$I_{\mu\nu}$                                                                                                                | $-I_{\mu\nu}$<br>$I_{\mu\nu}$<br>$I_{\mu\nu}$                                                                                                                        | $-I_{\mu\nu}$<br>$I_{\mu\nu}$<br>$I_{\mu\nu}$                                                                                                                        | $+1$<br>$+1$<br>$+1$                                                         | $I_{\mu\nu}$<br>$-I_{\mu\nu}$<br>$I_{\mu\nu}$                                                                                                                       | $+1$<br>$-1$<br>$-1$                                                         |
|  | 9  | 1 |   | $\mu_q \bar{\chi}(y) \sigma_{\mu\lambda} C_{\lambda\nu}(y) \chi(y)$<br>$r\mu_q \bar{\chi}(y) \sigma_{\mu\lambda} C_{\lambda\nu}(y) \chi(y)$<br>$\mu_q \bar{\chi}(y) \sigma_{\mu\lambda} \tau^3 C_{\lambda\nu}(y) \chi(y)$<br>$r\mu_q \bar{\chi}(y) \sigma_{\mu\lambda} \tau^3 C_{\lambda\nu}(y) \chi(y)$<br>$\mu_q \bar{\chi}(y) \sigma_{\mu\lambda} \gamma_5 C_{\lambda\nu}(y) \chi(y)$<br>$r\mu_q \bar{\chi}(y) \sigma_{\mu\lambda} \gamma_5 C_{\lambda\nu}(y) \chi(y)$<br>$\mu_q \bar{\chi}(y) \sigma_{\mu\lambda} \gamma_5 \tau^3 C_{\lambda\nu}(y) \chi(y)$<br>$r\mu_q \bar{\chi}(y) \sigma_{\mu\lambda} \gamma_5 \tau^3 C_{\lambda\nu}(y) \chi(y)$                                                                                               | $I_{\mu\nu}$<br>$I_{\mu\nu}$<br>$-I_{\mu\nu}$<br>$-I_{\mu\nu}$<br>$-I_{\mu\nu}$<br>$-I_{\mu\nu}$<br>$I_{\mu\nu}$<br>$I_{\mu\nu}$<br>$I_{\mu\nu}$             | $I_{\mu\nu}$<br>$I_{\mu\nu}$<br>$-I_{\mu\nu}$<br>$-I_{\mu\nu}$<br>$-I_{\mu\nu}$<br>$-I_{\mu\nu}$<br>$I_{\mu\nu}$<br>$I_{\mu\nu}$<br>$I_{\mu\nu}$                     | $-I_{\mu\nu}$<br>$-I_{\mu\nu}$<br>$-I_{\mu\nu}$<br>$-I_{\mu\nu}$<br>$-I_{\mu\nu}$<br>$-I_{\mu\nu}$<br>$I_{\mu\nu}$<br>$I_{\mu\nu}$<br>$I_{\mu\nu}$                   | $+1$<br>$+1$<br>$+1$<br>$+1$<br>$+1$<br>$+1$<br>$+1$<br>$+1$<br>$+1$         | $-I_{\mu\nu}$<br>$I_{\mu\nu}$<br>$-I_{\mu\nu}$<br>$I_{\mu\nu}$<br>$I_{\mu\nu}$<br>$-I_{\mu\nu}$<br>$I_{\mu\nu}$<br>$I_{\mu\nu}$<br>$-I_{\mu\nu}$                    | $-1$<br>$-1$<br>$+1$<br>$+1$<br>$-1$<br>$-1$<br>$+1$<br>$+1$<br>$+1$         |
|  | 10 | 1 |   | $\bar{\chi}(y) t^a \chi(y) \bar{\chi}(y) t^a \chi(y)$<br>$\bar{\chi}(y) t^a \chi(y) \bar{\chi}(y) \tau^3 t^a \chi(y)$<br>$\bar{\chi}(y) \tau^3 t^a \chi(y) \bar{\chi}(y) \tau^3 t^a \chi(y)$<br>$\bar{\chi}(y) t^a \chi(y) \bar{\chi}(y) \gamma_5 t^a \chi(y)$<br>$\bar{\chi}(y) t^a \chi(y) \bar{\chi}(y) \gamma_5 \tau^3 t^a \chi(y)$<br>$\bar{\chi}(y) \tau^3 t^a \chi(y) \bar{\chi}(y) \gamma_5 t^a \chi(y)$<br>$\bar{\chi}(y) \tau^3 t^a \chi(y) \bar{\chi}(y) \gamma_5 \tau^3 t^a \chi(y)$<br>$\bar{\chi}(y) \gamma_5 t^a \chi(y) \bar{\chi}(y) \gamma_5 t^a \chi(y)$<br>$\bar{\chi}(y) \gamma_5 t^a \chi(y) \bar{\chi}(y) \gamma_5 \tau^3 t^a \chi(y)$<br>$\bar{\chi}(y) \gamma_5 \tau^3 t^a \chi(y) \bar{\chi}(y) \gamma_5 \tau^3 t^a \chi(y)$ | $I_{\mu\nu}$<br>$I_{\mu\nu}$<br>$I_{\mu\nu}$<br>$I_{\mu\nu}$<br>$I_{\mu\nu}$<br>$I_{\mu\nu}$<br>$I_{\mu\nu}$<br>$I_{\mu\nu}$<br>$I_{\mu\nu}$<br>$I_{\mu\nu}$ | $I_{\mu\nu}$<br>$I_{\mu\nu}$<br>$-I_{\mu\nu}$<br>$-I_{\mu\nu}$<br>$-I_{\mu\nu}$<br>$-I_{\mu\nu}$<br>$-I_{\mu\nu}$<br>$-I_{\mu\nu}$<br>$-I_{\mu\nu}$<br>$-I_{\mu\nu}$ | $-I_{\mu\nu}$<br>$I_{\mu\nu}$<br>$I_{\mu\nu}$<br>$-I_{\mu\nu}$<br>$-I_{\mu\nu}$<br>$-I_{\mu\nu}$<br>$-I_{\mu\nu}$<br>$-I_{\mu\nu}$<br>$-I_{\mu\nu}$<br>$-I_{\mu\nu}$ | $+1$<br>$+1$<br>$+1$<br>$+1$<br>$+1$<br>$+1$<br>$+1$<br>$+1$<br>$+1$<br>$+1$ | $I_{\mu\nu}$<br>$-I_{\mu\nu}$<br>$I_{\mu\nu}$<br>$-I_{\mu\nu}$<br>$I_{\mu\nu}$<br>$-I_{\mu\nu}$<br>$-I_{\mu\nu}$<br>$-I_{\mu\nu}$<br>$-I_{\mu\nu}$<br>$-I_{\mu\nu}$ | $-1$<br>$-1$<br>$+1$<br>$+1$<br>$-1$<br>$-1$<br>$+1$<br>$+1$<br>$+1$<br>$+1$ |
|  | 11 | 1 |   | $\bar{\chi}(y) \gamma_\mu t^a \chi(y) \bar{\chi}(y) \gamma_\nu t^a \chi(y)$<br>$\bar{\chi}(y) \gamma_\mu t^a \chi(y) \bar{\chi}(y) \gamma_\nu \tau^3 t^a \chi(y)$<br>$\bar{\chi}(y) \gamma_\mu \tau^3 t^a \chi(y) \bar{\chi}(y) \gamma_\nu \tau^3 t^a \chi(y)$<br>$\bar{\chi}(y) \gamma_\mu t^a \chi(y) \bar{\chi}(y) \gamma_\nu \tau^3 t^a \chi(y)$<br>$\bar{\chi}(y) \gamma_\mu \tau^3 t^a \chi(y) \bar{\chi}(y) \gamma_\nu \tau^3 t^a \chi(y)$                                                                                                                                                                                                                                                                                                      | $I_{\mu\nu}$<br>$I_{\mu\nu}$<br>$I_{\mu\nu}$<br>$I_{\mu\nu}$<br>$I_{\mu\nu}$                                                                                 | $I_{\mu\nu}$<br>$I_{\mu\nu}$<br>$-I_{\mu\nu}$<br>$-I_{\mu\nu}$<br>$-I_{\mu\nu}$                                                                                      | $-I_{\mu\nu}$<br>$I_{\mu\nu}$<br>$I_{\mu\nu}$<br>$-I_{\mu\nu}$<br>$-I_{\mu\nu}$                                                                                      | $+1$<br>$+1$<br>$+1$<br>$+1$<br>$+1$                                         | $I_{\mu\nu}$<br>$-I_{\mu\nu}$<br>$I_{\mu\nu}$<br>$-I_{\mu\nu}$<br>$-I_{\mu\nu}$                                                                                     | $+1$<br>$-1$<br>$+1$<br>$+1$<br>$+1$                                         |
|  |    |   |   |                                                                                                                                                                                                                                                                                                                                                                                                                                                                                                                                                                                                                                                                                                                                                        |                                                                                                                                                              |                                                                                                                                                                      |                                                                                                                                                                      |                                                                              | cf. 6, 7                                                                                                                                                            |                                                                              |
